# Supplementary material for: Unboundedness and Downward Closures of Higher-Order Pushdown Automata
Source: arXiv:1507.03304 source file (2015-11-05)
Supplement: Supplementary file 1 [file popl-appendix.tex]

\section{Proofs for the Single Character Case}

\subsection{Proof of Lemma~\ref{lem:branch-runs}}
\input{branch-runs-proof}

\subsection{Proof of Lemma~\ref{lem:sim-to-pda}}
\input{sim-to-pda-proof}

\section{Proofs for the General Case}

\subsection{Proof of Theorem~\ref{thm:no-tests-sim}}
\input{no-tests-sim-proof}

\subsection{Decidability at Order-$0$}

We give the complete definitions and proof of the decidability at order-$0$.

\input{decidability-order-0-proof}

\subsection{Proof of Lemma~\ref{lem:branch-runs-sim}}
\input{branch-runs-sim-proof}

\subsection{Proof of Lemma~\ref{lem:sim-to-pda-sim}}
\input{sim-to-pda-sim-proof}
